# Supplementary material for: Expected seismicity and the seismic noise environment of Europa
Source: arXiv:1705.03424 source file (2017-08-01)
Supplement: Supplementary file 1 [file agutmpl_-_Supporting_Information.pdf]

# Supporting Information for "Expected seismicity and the seismic noise environment of Europa"

## Contents of this file

1. Introduction to included audio files

## Additional Supporting Information (Files uploaded separately)

1. Captions for Audio S1 to S3

## Introduction

Three sound files are included in WAV format. All 3 are produced by speeding up synthetic seismic records by a factor of 500 using Matlab tools available from Zhigang Peng [http://geophysics.eas.gatech.edu/people/zpeng/EQ_Music/, *Kilb et al.*, 2012].

## Text S1.

**Audio S1.** 22 second file compressed from 3 hours of continuous data based on the model D seismicity catalog in the model with a 5 km thick ice shell and high Q.

**Audio S2.** The same time window as S1 but in the 20 km thick ice shell model with high Q.

**Audio S3.** An example in the 5 km, high Q model, also including the ocean noise modeled in section 6.3.

---

## References

Kilb, D., Z. Peng, D. Simpson, A. Michael, M. Fisher, and D. Rohrlick (2012), Listen, watch, learn: SeisSound video products, *Seis. Res. Lett.*, *83*(2), 281–286, doi: 10.1785/gssrl.83.2.281.
